# Supplementary material for: ConceptLens: from Pixels to Understanding
Source: arXiv:2410.05311 source file (2024-10-04)
Supplement: Supplementary file 1 [file appendix.tex]

\appendix
\section{Appendices}
% \renewcommand\chaptername{Appendix}
% \chapter{A}
\label{appendix}
%\vspace{-4.0cm}

\subsection{Related work}
\label{sec:literature_review}

Efforts to demystify deep learning~\cite{gunning2019xai,adadi2018peeking,minh2022explainable} are ongoing. Methods for explainability can be categorized based on their approach to understanding input data, such as feature summarization~\cite{selvaraju2016grad,lime_rebeiro}, or the model's internal representation, like node summarization~\cite{zhou2018interpreting,bau2020understanding}. These methods further classify into model-specific~\cite{selvaraju2016grad} or model-agnostic~\cite{lime_rebeiro} approaches. Some methods rely on human interpretation of explanatory data, such as posing counterfactual questions~\cite{DBLP:journals/corr/abs-1711-00399}.

Model-agnostic techniques for feature attribution, such as LIME~\cite{lime_rebeiro} and SHAP~\cite{shap_lundberg}, aim to elucidate model predictions by assessing the influence of individual features. However, they encounter challenges like explanation instability~\cite{attacklime_alvarez} and susceptibility to biased classifiers~\cite{attacklimeandshap_lakkaraju}. On the other hand, pixel attribution endeavors to comprehend predictions by assigning significance to individual pixels~\cite{saliencymap_simonyan,gradcam_batra,smoothgrad_smilkov}. Nonetheless, it faces notable limitations, particularly with ReLU activation~\cite{gradcamattack_shrikumar} and adversarial perturbations~\cite{unreliablepixelattribution_kim}, leading to inconsistencies in interpretability.

Explanations developed by \cite{tcav_kim,tcar_crabbe} employ supervised learning and curated concepts. These methods utilize classifiers on target concepts, with weights representing Concept Activation Vectors (CAVs). Another approach by \cite{ace_ghorbani} utilizes image segmentation and clustering for concept selection, albeit potentially losing information and only applicable to visible concepts. \cite{invertibletcav_zhang} proposed enhancements using Non-negative Matrix Factorization to mitigate information loss. Individual Conditional Expectation (ICE) plots~\cite{ice_goldstein} and Partial Dependency Plots~\cite{pdp_friedman} provide insights into prediction-feature relationships from both local and global perspectives but may struggle with intricate feature interactions.

Previous studies suggest that hidden neurons may represent high-level concepts~\cite{zhou2018interpreting,bau2020understanding}, but these methods often require semantic segmentation~\cite{xiao2018unified} (resource-intensive) or explicit concept annotations~\cite{tcav_kim}. 

Some research have utilized Semantic Web data for explaining deep learning models~\cite{confalonieri2021using,diaz2022explainable}, and Concept Induction for providing explanations~\cite{sarker2017explaining,9736291}. However, their focus was on analyzing input-output behavior, generating explanations for the overall system. 
% In contrast, we concentrate on understanding internal node activations.

CLIP-Dissect~\cite{oikarinen2022clip} represents work similar to ours, employing a different approach. They utilize the CLIP pre-trained model, employing zero-shot learning to associate images with labels. Label-Free Concept Bottleneck Models~\cite{oikarinen2023label}, building upon CLIP-Dissect, use GPT-4~\cite{achiam2023gpt} for concept set generation.
However, CLIP-Dissect has limitations that may be challenging to overcome without significant changes to the approach. These include limited accuracy in predicting output labels based on concepts in the last hidden layer and difficulty in transferring to other modalities or domain-specific applications. The Label-Free approach inherits these limitations and may compromise explainability, as it uses a concept derivation method that is not inherently explainable.

%\pagebreak

\subsection{Details of AMT user-study}
\label{subsec:appendix_amt}
Using a subset of randomly chosen 1050 ADE20K images, we conducted a user study through Amazon Mechanical Turk using the Cloud Research platform, to annotate images based on a list of concepts derived from Table\ref{tab:appendix_listofConcepts_google}. 

The study protocol was reviewed and approved by the Institutional Review Board (IRB) at Kansas State University and was deemed exempt under the criteria outlined in the Federal Policy for the Protection of Human Subjects, 45 CFR §104(d), category: Exempt Category 2 Subsection ii. The study was conducted in 35 batches (each batch containing 30 images), with 5 participants per study compensated with \$5 for completing the task. The task was estimated to take approximately 40 minutes, equivalent to \$7.50 per hour. 

For each image, users were presented with a list of concepts (a concise form of concepts from 
Table~\ref{tab:appendix_listofConcepts_google}) to choose from, including buffet, building, building and dome, central\_reservation, clamp\_lamp and clamp, closet and air-conditioning, cross\_walk, edifice and skyscraper, faucet and flusher, field, flusher and soap\_dish, footboard and chain, hedgerow and hedge, lid and soap\_dispenser, mountain, mountain and bushes, night\_table, open\_fireplace and coffee\_table, pillow, potty and flusher, road, road and automobile, road and car, route, route and car, shower\_stall and cistern, Shower\_stall and screen\_door, skyscraper, slope, tap and crapper, tap and shower\_screen, teapot and saucepan, wardrobe and air-conditioning. 

Users were allowed to select multiple concepts for each image, indicating all concepts that applied to the given image. These selected concepts were considered annotations for the respective image.

\subsection{Detailed result of Non-TLA  and Statistical Evaluation}
The detailed results of Non-target Label Activation Percentages (Non-TLA) for the Google dataset are meticulously outlined in Table \ref{tab:appendix_listofConcepts_google}. This table presents a carefully curated selection, focusing on concepts and neuron ensembles with Target Label Activation (TLA) exceeding 80\%. It offers valuable insights into the percentage of Non-Target Label images activating the neuron(s) associated with the concept under scrutiny across a spectrum of activation thresholds.

Furthermore, Table \ref{tab:appendix_non_targ_ade_google} compares the Non-TLA between the ADE20K and Google Image datasets, highlighting variations in activation across different thresholds and providing a comprehensive view of dataset-specific nuances.

Lastly, the statistical evaluation for \textit{confirmed} concepts, outlined in Table \ref{tab:appendix_stats_eval}, underscores concepts where statistical significance (with a $p$-value less than 0.05 for the MWU test) has been established. This table offers insights into the percentage of non-target label images activating the associated neuron(s) across diverse activation thresholds, providing valuable information on the robustness of the identified concepts across both the Google and ADE20K datasets.

\begin{table}[p]
\caption{Non-target Label Activation Percentages (Non-TLA) for Google dataset: The table showcases a refined selection, inclusive of concepts and neuron ensembles with targ(et) activation $>$ 80\%. Non-t: percentage of non-target images that activate the neuron(s) associated with the concept being analyzed across various activation thresholds.}
\label{tab:appendix_listofConcepts_google}
\centering
\resizebox{\columnwidth}{!}{
\begin{footnotesize}
\begin{tabular}{lr|r|rr|rr}
\hline
Concepts & Neuron & \textbf{targ \%$>$0} & \multicolumn{4}{c}{Non-target \% for different threshold values} \\
\hline
\multicolumn{2}{c}{} &  & non-t $>$0 & non-t $>$ 20\% & non-t $>$ 40\% & non-t $>$ 60\%\\
\hline
buffet & 62 & \textbf{83.607} & 32.714 & 12.374 & 3.708 & 0.825 \\
building & 0 & \textbf{89.024} & 72.328 & 39.552 & 12.040 & 2.276 \\
building & 0, 63 & \textbf{80.164} & 43.375 & 12.314 & 2.276 & 0.182 \\
building and dome & 0 & \textbf{90.400} & 78.185 & 45.133 & 14.643 & 2.639 \\
central\_reservation & 43 & \textbf{95.541} & 84.973 & 57.993 & 19.734 & 2.913 \\
\hline
clamp\_lamp and clamp & 7 & \textbf{95.139} & 59.504 & 29.229 & 9.000 & 1.652 \\
closet and air\_conditioning & 19 & \textbf{86.891} & 71.054 & 38.491 & 10.135 & 1.267 \\
cross\_walk & 1 & \textbf{88.770} & 28.241 & 6.800 & 1.524 & 0.521 \\
edifice and skyscraper & 63 & \textbf{92.135} & 48.761 & 21.786 & 8.379 & 2.229 \\
faucet and flusher & 29 & \textbf{95.695} & 78.562 & 37.862 & 12.104 & 1.873 \\
\hline
field & 18 & \textbf{91.824} & 65.333 & 30.207 & 8.183 & 1.656 \\
flusher and soap\_dish & 56 & \textbf{90.094} & 63.552 & 29.901 & 7.695 & 1.148 \\
footboard and chain & 49 & \textbf{88.889} & 66.702 & 40.399 & 17.064 & 4.399 \\
hedgerow and hedge & 54 & \textbf{91.165} & 68.527 & 30.421 & 7.685 & 1.352 \\
lid and soap\_dispenser & 29 & \textbf{99.237} & 78.571 & 34.989 & 9.052 & 1.485 \\
\hline
mountain and bushes & 16 & \textbf{87.037} & 24.969 & 10.424 & 4.666 & 1.937 \\
mountain and bush & 16 & \textbf{87.037} & 24.969 & 10.424 & 4.666 & 1.937 \\
mountain & 43 & \textbf{99.367} & 88.516 & 64.169 & 23.112 & 4.326 \\
night\_table & 3 & \textbf{90.446} & 56.714 & 27.691 & 7.691 & 1.137 \\
open\_fireplace and coffee\_table & 41 & \textbf{88.525} & 16.381 & 4.325 & 0.812 & 0.088 \\
\hline
pillow & 3 & \textbf{98.214} & 61.250 & 28.228 & 7.249 & 1.001 \\
pillow & 50 & \textbf{99.405} & 66.834 & 24.242 & 4.101 & 0.530 \\
pillow & 3, 50 & \textbf{97.605} & 46.492 & 9.634 & 0.988 & 0.049 \\
potty and flusher & 29 & \textbf{88.525} & 76.830 & 36.537 & 10.755 & 1.932 \\
road and car & 51 & \textbf{98.810} & 48.571 & 25.373 & 8.399 & 3.261 \\
\hline
road and automobile & 51 & \textbf{92.560} & 41.466 & 16.055 & 3.301 & 0.701 \\
road & 48 & \textbf{100.000} & 76.789 & 47.897 & 18.843 & 3.803 \\
road & 48, 51 & \textbf{97.099} & 44.592 & 17.727 & 3.471 & 0.702 \\
route & 48 & \textbf{100.000} & 80.834 & 51.873 & 21.034 & 4.979 \\
route and car & 51 & \textbf{92.628} & 47.408 & 18.871 & 4.081 & 1.416 \\
\hline
route & 48, 51 & \textbf{94.334} & 45.089 & 18.937 & 4.809 & 1.169 \\
shower\_stall and cistern & 8 & \textbf{100.000} & 53.186 & 24.788 & 8.485 & 1.372 \\
Shower\_stall and screen\_door & 57 & \textbf{98.496} & 31.747 & 12.876 & 4.121 & 1.026 \\
slope & 18 & \textbf{92.143} & 64.503 & 29.976 & 6.894 & 1.200 \\
tap and crapper & 36 & \textbf{89.130} & 70.606 & 36.839 & 13.696 & 2.511 \\
\hline
tap and shower\_screen & 36 & \textbf{86.250} & 72.584 & 32.574 & 7.836 & 0.860 \\
teapot and saucepan & 30 & \textbf{81.481} & 47.984 & 18.577 & 4.367 & 0.845 \\
wardrobe and air\_conditioning & 19 & \textbf{89.091} & 65.034 & 31.795 & 6.958 & 1.145\\
skyscraper & 22 & \textbf{99.359} & 54.893 & 21.914 & 0.977 & 0.977 \\
skyscraper & 54 & \textbf{98.718} & 70.432 & 26.851 & 7.050 & 0.941 \\
\hline
skyscraper & 63 & \textbf{94.393} & 51.612 & 20.618 & 5.775 & 1.143 \\
skyscraper & 22, 26 & \textbf{82.116} & 22.274 & 3.423 & 0.292 & 0.004 \\
skyscraper & 26, 54 & \textbf{82.225} & 28.782 & 5.444 & 0.703 & 0.054 \\
skyscraper & 22, 54 & \textbf{97.165} & 47.422 & 7.910 & 0.465 & 0.000 \\
skyscraper & 22, 63 & \textbf{96.947} & 36.408 & 5.521 & 0.449 & 0.008 \\
\hline
skyscraper & 26, 63 & \textbf{81.788} & 21.421 & 3.335 & 0.534 & 0.088 \\
skyscraper & 54, 63 & \textbf{96.074} & 37.149 & 5.594 & 0.615 & 0.046 \\
skyscraper & 22, 26, 54 & \textbf{81.461} & 18.940 & 2.363 & 0.169 & 0.000 \\
skyscraper & 22, 26, 63 & \textbf{81.243} & 15.252 & 1.706 & 0.184 & 0.004 \\
skyscraper & 22, 54, 63 & \textbf{95.420} & 29.090 & 3.023 & 0.234 & 0.000 \\
skyscraper & 26, 54, 63 & \textbf{81.134} & 16.823 & 1.975 & 0.350 & 0.023 \\
skyscraper & 22, 26, 54, 63 & \textbf{80.589} & 13.093 & 0.872 & 0.015 & 0.000 \\
\hline
\end{tabular}
\end{footnotesize}}
\end{table}

%\subsection{Detailed result of Non-TLA\% for Google and ADE20K dataset}
\begin{table}[p]
\caption{Non-target Label Activation Percentages (Non-TLA) for ADE20K and Google Image dataset: Non-t: percentage of non-target label images that activate the neuron(s) associated with the concept being analyzed across various activation thresholds.}
\label{tab:appendix_non_targ_ade_google}
\centering
\resizebox{\columnwidth}{!}{
\begin{footnotesize}
\begin{tabular}{l|rr|rr|rr|rr}
\hline
Concepts & \multicolumn{2}{c}{non-t $>$0} & \multicolumn{2}{c}{non-t $>$20\%} & \multicolumn{2}{c}{non-t $>$40\%} & \multicolumn{2}{c}{non-t $>$60\%}\\
\hline
 & google & ADE20K & google & ADE20K & google & ADE20K & google & ADE20K\\
\hline
buffet & 32.714 & 40.135 & 12.374 & 25.817 & 3.708 & 9.470 & 0.825 & 1.804 \\
building & 43.375 & 11.458 & 12.314 & 5.208 & 2.276 & 1.458 & 0.182 & 0.000 \\
building and dome & 78.185 & 26.170 & 45.133 & 5.893 & 14.643 & 0.867 & 2.639 & 0.000 \\
central\_reservation & 84.973 & 44.893 & 57.993 & 34.343 & 19.734 & 14.927 & 2.913 & 3.816 \\
clamp\_lamp and clamp & 59.504 & 27.273 & 29.229 & 19.170 & 9.000 & 8.300 & 1.652 & 1.976 \\
closet and air\_conditioning & 71.054 & 30.168 & 38.491 & 15.620 & 10.135 & 5.513 & 1.267 & 1.378 \\
cross\_walk & 28.241 & 21.474 & 6.800 & 16.391 & 1.524 & 9.784 & 0.521 & 2.922 \\
edifice and skyscraper & 48.761 & 24.187 & 21.786 & 8.453 & 8.379 & 1.300 & 2.229 & 0.260 \\
faucet and flusher & 78.562 & 56.967 & 37.862 & 30.580 & 12.104 & 11.097 & 1.873 & 1.850 \\
field & 65.333 & 66.161 & 30.207 & 30.043 & 8.183 & 10.412 & 1.656 & 2.386 \\
flusher and soap\_dish & 63.552 & 19.481 & 29.901 & 10.035 & 7.695 & 3.896 & 1.148 & 0.236 \\
footboard and chain & 66.702 & 27.975 & 40.399 & 13.671 & 17.064 & 5.063 & 4.399 & 1.013 \\
hedgerow and hedge & 68.527 & 45.120 & 30.421 & 28.390 & 7.685 & 13.308 & 1.352 & 2.028 \\
lid and soap\_dispenser & 78.571 & 57.512 & 34.989 & 18.427 & 9.052 & 2.817 & 1.485 & 0.352 \\
mountain & 88.516 & 45.144 & 64.169 & 33.725 & 23.112 & 16.115 & 4.326 & 3.842 \\
mountain and bushes & 24.969 & 28.331 & 10.424 & 16.573 & 4.666 & 6.607 & 1.937 & 1.904 \\
night\_table & 56.714 & 30.534 & 27.691 & 15.267 & 7.691 & 5.954 & 1.137 & 1.679 \\
open\_fireplace and coffee\_table & 16.381 & 26.139 & 4.325 & 10.590 & 0.812 & 2.413 & 0.088 & 0.268 \\
pillow & 46.492 & 12.500 & 9.634 & 3.869 & 0.988 & 1.190 & 0.049 & 0.149 \\
potty and flusher & 76.830 & 58.410 & 36.537 & 24.194 & 10.755 & 4.608 & 1.932 & 1.152 \\
road & 44.592 & 8.501 & 17.727 & 6.955 & 3.471 & 4.328 & 0.702 & 0.927 \\
road and automobile & 41.466 & 17.604 & 16.055 & 14.497 & 3.301 & 8.728 & 0.701 & 2.811 \\
road and car & 48.571 & 14.815 & 25.373 & 11.704 & 8.399 & 6.074 & 3.261 & 1.333 \\
route & 45.089 & 12.349 & 18.937 & 10.241 & 4.809 & 5.723 & 1.169 & 1.807 \\
route and car & 47.408 & 17.073 & 18.871 & 14.204 & 4.081 & 7.461 & 1.416 & 2.152 \\
shower\_stall and cistern & 53.186 & 25.982 & 24.788 & 9.700 & 8.485 & 4.965 & 1.372 & 1.039 \\
Shower\_stall and screen\_door & 31.747 & 24.910 & 12.876 & 14.320 & 4.121 & 5.897 & 1.026 & 1.203 \\
skyscraper & 13.093 & 3.009 & 0.872 & 0.463 & 0.015 & 0.231 & 0.000 & 0.116 \\
slope & 64.503 & 66.520 & 29.976 & 29.967 & 6.894 & 9.879 & 1.200 & 1.976 \\
tap and crapper & 70.606 & 62.225 & 36.839 & 12.861 & 13.696 & 4.890 & 2.511 & 0.611 \\
tap and shower\_screen & 72.584 & 62.621 & 32.574 & 13.180 & 7.836 & 4.733 & 0.860 & 0.607 \\
teapot and saucepan & 47.984 & 23.632 & 18.577 & 11.176 & 4.367 & 6.519 & 0.845 & 1.281 \\
wardrobe and air\_conditioning & 65.034 & 30.525 & 31.795 & 16.160 & 6.958 & 5.525 & 1.145 & 0.967\\

\hline
\end{tabular}
\end{footnotesize}}
\end{table}

%\subsection{Detailed result of Statistical Evaluation}
\begin{table}[p]
\caption{Statistical Evaluation for \textit{confirmed} concepts (concepts getting $p$-value $<$0.05 for MWU): Non-t: percentage of non-target label images activating the associated neuron(s) analyzed across various activation thresholds.}
\label{tab:appendix_stats_eval}
\centering
\resizebox{.70\columnwidth}{!}{
\begin{footnotesize}
\begin{tabular}{l|rr|r}
\hline
Concepts & Google & ADE20K & p-values\\
\hline
\hline
 & \multicolumn{2}{c}{\textbf{non-t $>$0}} & \\
\hline
building & 43.37468 & 11.45833 & 0.018471 \\
building and dome & 78.185 & 26.16984 & 6.06E-05 \\
central\_reservation & 84.97336 & 44.89338 & 1.75E-66 \\
closet and air\_conditioning & 71.05416 & 30.16845 & 0.009373 \\
edifice and skyscraper & 48.76092 & 24.18726 & 0.016058 \\
faucet and flusher & 78.562 & 56.96671 & 9.19E-07 \\
footboard and chain & 66.702 & 27.97468 & 0.000284 \\
lid and soap\_dispenser & 78.57143 & 57.51174 & 0.00218 \\
pillow & 46.49232 & 12.5 & 4.21E-23 \\
potty and flusher & 76.82974 & 58.41014 & 1.39E-07 \\
shower\_stall and cistern & 53.1865 & 25.98152 & 0.016657 \\
tap and crapper & 70.60579 & 62.22494 & 6.17E-08 \\
tap and shower\_screen & 72.584 & 62.62136 & 0.007024 \\
\hline
\multicolumn{3}{c}{\textbf{Wilcoxon signed rank test (non-t $>$0)}} & \textbf{0.0001221}\\
\hline
\hline
 & \multicolumn{2}{c}{\textbf{non-t $>$20 \%}} & \\
\hline
 building & 12.31365 & 5.208333 & 1.72E-17 \\
building and dome & 45.13343 & 5.892548 & 1.37E-23 \\
clamp\_lamp and clamp & 29.2287 & 19.16996 & 1.57E-07 \\
closet and air\_conditioning & 38.4913 & 15.62021 & 0.000287 \\
edifice and skyscraper & 21.78641 & 8.452536 & 5.80E-17 \\
faucet and flusher & 37.86209 & 30.57953 & 1.80E-15 \\
lid and soap\_dispenser & 34.98939 & 18.42723 & 2.74E-15 \\
mountain and bushes & 10.42437 & 16.57335 & 3.25E-06 \\
pillow & 9.634389 & 3.869048 & 3.49E-49 \\
potty and flusher & 36.53659 & 24.19355 & 3.69E-18 \\
Shower\_stall and screen\_door & 12.87584 & 14.3201 & 0.035051 \\
skyscraper & 0.872071 & 0.462963 & 1.99E-05 \\
tap and crapper & 36.83933 & 12.86064 & 0.000114 \\
tap and shower\_screen & 32.5745 & 13.17961 & 3.22E-14 \\
wardrobe and air\_conditioning & 31.79496 & 16.16022 & 2.18E-11\\
\hline
\multicolumn{3}{c}{\textbf{Wilcoxon signed rank test (non-t $>$ 20\%)}} & \textbf{0.0004272}\\
\hline
\hline
 & \multicolumn{2}{c}{\textbf{non-t $>$40 \%}} & \\
\hline
building & 2.27609 & 1.458333 & 3.16E-19 \\
building and dome & 14.64338 & 0.866551 & 6.28E-20 \\
central\_reservation & 19.73357 & 14.92705 & 1.18E-05 \\
clamp\_lamp and clamp & 9.000096 & 8.300395 & 2.79E-31 \\
closet and air\_conditioning & 10.1354 & 5.513017 & 6.38E-09 \\
cross\_walk & 1.52392 & 9.78399 & 0.000572 \\
edifice and skyscraper & 8.37939 & 1.30039 & 5.06E-17 \\
faucet and flusher & 12.10377 & 11.09741 & 2.90E-24 \\
field & 8.183384 & 10.41215 & 3.82E-05 \\
flusher and soap\_dish & 7.695067 & 3.896104 & 4.26E-08 \\
lid and soap\_dispenser & 9.052334 & 2.816901 & 2.04E-19 \\
mountain and bushes & 4.666314 & 6.606943 & 1.28E-12 \\
pillow & 0.988239 & 1.190476 & 1.37E-23 \\
potty and flusher & 10.75519 & 4.608295 & 1.97E-09 \\
road & 3.471037 & 4.327666 & 0.033105 \\
road and car & 8.399088 & 6.074074 & 0.009958 \\
Shower\_stall and screen\_door & 4.120976 & 5.89651 & 1.13E-07 \\
skyscraper & 0.015367 & 0.231481 & 2.47E-30 \\
slope & 6.893903 & 9.879254 & 1.14E-07 \\
tap and shower\_screen & 7.835857 & 4.73301 & 2.05E-12 \\
wardrobe and air\_conditioning & 6.9579 & 5.524862 & 1.70E-19\\
\hline
\multicolumn{3}{c}{\textbf{Wilcoxon signed rank test (non-t $>$ 40\%)}} & \textbf{0.0479}\\
\hline
% \hline
%  & \multicolumn{2}{c}{\textbf{non-t $>$60 \%}} & \\
% \hline
% building & 0.182087 & 0 & 1.08E-07 \\
% building and dome & 2.639495 & 0 & 5.70E-10 \\
% central\_reservation & 2.912966 & 3.815937 & 1.50E-07 \\
% clamp\_lamp and clamp & 1.652099 & 1.976285 & 4.24E-19 \\
% closet and air\_conditioning & 1.266925 & 1.378254 & 2.50E-07 \\
% cross\_walk & 0.520833 & 2.92249 & 0.000171 \\
% edifice and skyscraper & 2.228561 & 0.260078 & 4.80E-07 \\
% faucet and flusher & 1.872623 & 1.849568 & 0.008524 \\
% field & 1.655819 & 2.386117 & 1.43E-09 \\
% flusher and soap\_dish & 1.147982 & 0.236128 & 3.03E-13 \\
% lid and soap\_dispenser & 1.485149 & 0.352113 & 3.10E-07 \\
% mountain and bushes & 1.936961 & 1.903695 & 9.96E-12 \\
% pillow & 0.048848 & 0.14881 & 1.04E-09 \\
% potty and flusher & 1.931664 & 1.152074 & 0.010232 \\
% road & 0.701794 & 0.927357 & 0.000445 \\
% road and car & 3.261441 & 1.333333 & 3.79E-05 \\
% route and car & 1.415601 & 2.15208 & 0.000137 \\
% shower\_stall and cistern & 1.372089 & 1.039261 & 0.031085 \\
% Shower\_stall and screen\_door & 1.025822 & 1.203369 & 9.36E-11 \\
% skyscraper & 0 & 0.115741 & 6.15E-26 \\
% slope & 1.200192 & 1.975851 & 2.39E-10 \\
% tap and shower\_screen & 0.859795 & 0.606796 & 3.67E-08 \\
% wardrobe and air\_conditioning & 1.144971 & 0.966851 & 1.52E-14\\
\hline
\end{tabular}
\end{footnotesize}}
\end{table}

\begin{table}[p]
% \caption{Non-target activations for both ADE20K and Google dataset: Non-t: percentage of non-target images activating the associated neuron(s) analyzed across various activation thresholds.}
% \label{tab:non_targ_ade_google}
\centering
\resizebox{.70\columnwidth}{!}{
\begin{footnotesize}
\begin{tabular}{l|rr|r}
\hline
 & \multicolumn{2}{c}{\textbf{non-t $>$ 60\%}} & \\
\hline
building & 0.182087 & 0 & 1.08E-07 \\
building and dome & 2.639495 & 0 & 5.70E-10 \\
central\_reservation & 2.912966 & 3.815937 & 1.50E-07 \\
clamp\_lamp and clamp & 1.652099 & 1.976285 & 4.24E-19 \\
closet and air\_conditioning & 1.266925 & 1.378254 & 2.50E-07 \\
cross\_walk & 0.520833 & 2.92249 & 0.000171 \\
edifice and skyscraper & 2.228561 & 0.260078 & 4.80E-07 \\
faucet and flusher & 1.872623 & 1.849568 & 0.008524 \\
field & 1.655819 & 2.386117 & 1.43E-09 \\
flusher and soap\_dish & 1.147982 & 0.236128 & 3.03E-13 \\
lid and soap\_dispenser & 1.485149 & 0.352113 & 3.10E-07 \\
mountain and bushes & 1.936961 & 1.903695 & 9.96E-12 \\
pillow & 0.048848 & 0.14881 & 1.04E-09 \\
potty and flusher & 1.931664 & 1.152074 & 0.010232 \\
road & 0.701794 & 0.927357 & 0.000445 \\
road and car & 3.261441 & 1.333333 & 3.79E-05 \\
route and car & 1.415601 & 2.15208 & 0.000137 \\
shower\_stall and cistern & 1.372089 & 1.039261 & 0.031085 \\
Shower\_stall and screen\_door & 1.025822 & 1.203369 & 9.36E-11 \\
skyscraper & 0 & 0.115741 & 6.15E-26 \\
slope & 1.200192 & 1.975851 & 2.39E-10 \\
tap and shower\_screen & 0.859795 & 0.606796 & 3.67E-08 \\
wardrobe and air\_conditioning & 1.144971 & 0.966851 & 1.52E-14\\
\hline
\multicolumn{3}{c}{\textbf{Wilcoxon signed rank test (non-t $>$ 60\%)}} & \textbf{0.05803}\\
\hline
\end{tabular}
\end{footnotesize}}
\end{table}
